# Supplementary material for: Spin-orbit torques and their associated effective fields from gigahertz to terahertz
Source: arXiv:1906.11314 ancillary file (2020-12-18)
Supplement: Supplementary file 1 [file Supplementary.pdf]

## SUPPLEMENTARY FIGURES

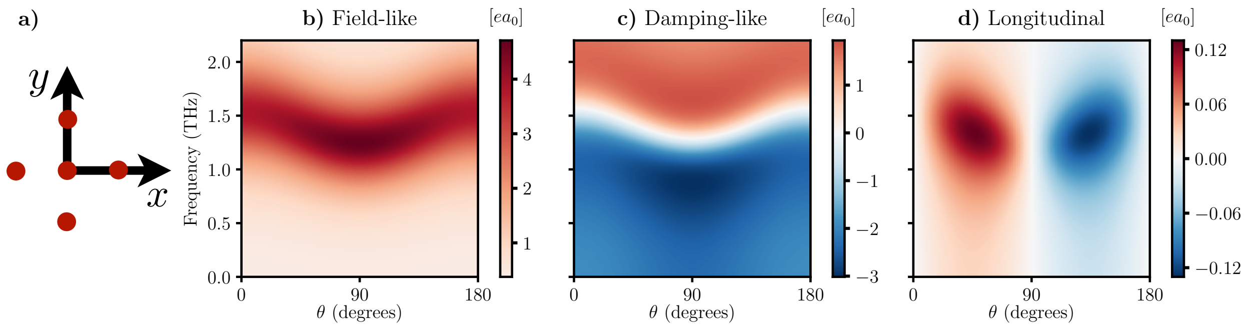


**Supplementary Figure 1** | Frequency and angular dependencies of the dynamical spin-orbit torques $\boldsymbol{\tau}^{\mathrm{SOT}}$ in-phase with the oscillatory electric field when the magnetic moment of the ferromagnetic layer in the Co/Pt(001) bilayer is rotated within the $zx$ plane by an external magnetic field. This system presents an out-of-plane magnetic anisotropy, with the four-fold symmetric magnetic square lattice formed by Co depicted in (a). $z$ is the normal to the film surface and the electric field is applied along $x$, with $\theta$ the angle between the magnetic moment and the surface normal. The torques are obtained in units of $ea_0 = 8.48 \times 10^{-30}\,\mathrm{C\,m}$, where $e$ is the electronic charge and $a_0$ is the Bohr radius. The torque vector was decomposed into the local frame of reference given by: (b) a field-like component along $\hat{\mathbf{m}}_{\mathrm{Fe}} \times \delta\hat{\mathbf{s}}$; (c) a damping-like component along $\hat{\mathbf{m}}_{\mathrm{Fe}} \times (\hat{\mathbf{m}}_{\mathrm{Fe}} \times \delta\hat{\mathbf{s}})$; and (d) a longitudinal contribution along $\hat{\mathbf{m}}_{\mathrm{Fe}}$.

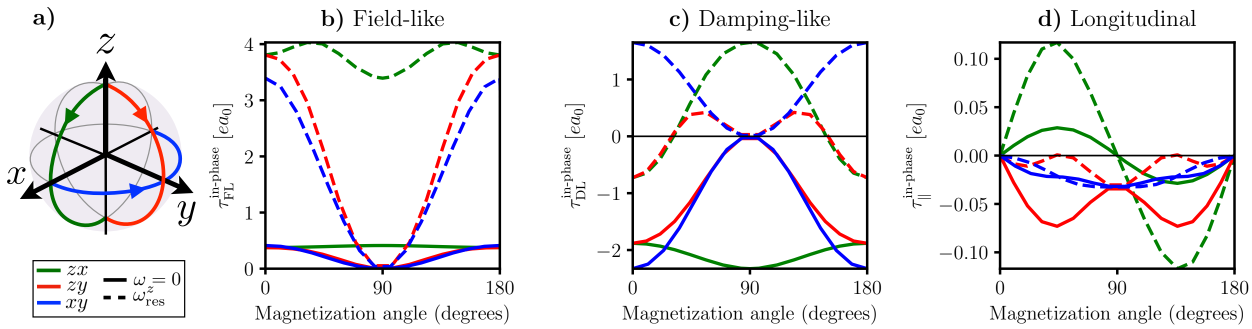


**Supplementary Figure 2** | Angular dependencies of spin-orbit torques in Co/Pt(001) that are in-phase with the oscillatory electric field along the directions indicated in (a): $z \to x$ (green), $z \to y$ (red) and $x \to y$ (blue). The torques are decomposed in (b) field-like, (c) damping-like and (d) longitudinal components for two distinct frequencies: static limit $\omega = 0$ (solid lines) and $\omega^z_{\text{res}} = 1.5\,\text{THz}$ (dashed lines). The torques are given in units of $ea_0 = 8.48 \times 10^{-30}\,\text{C m}$, where $e$ is the electronic charge and $a_0$ is the Bohr radius.

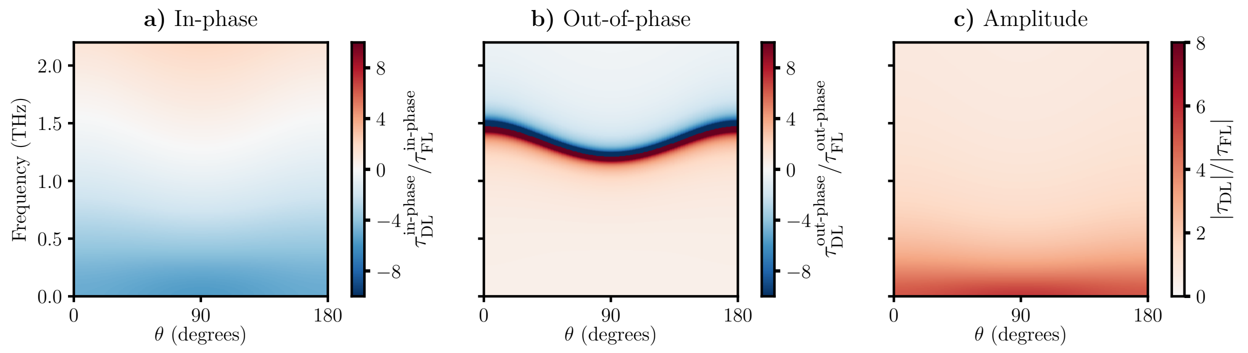


**Supplementary Figure 3** | Ratios between damping-like and field-like components of the spin-orbit torques in Co/Pt(001). Frequency and angular dependencies of the ratios between the damping-like, $\tau_{\text{DL}}(\omega)$, and field-like, $\tau_{\text{FL}}(\omega)$, components of the spin-orbit torques: (a) in-phase and (b) out-of-phase contributions, and (c) amplitudes. The magnetic moment is rotated in the $zx$ plane, $z$ is the normal to the film surface and the electric field is applied along $x$.

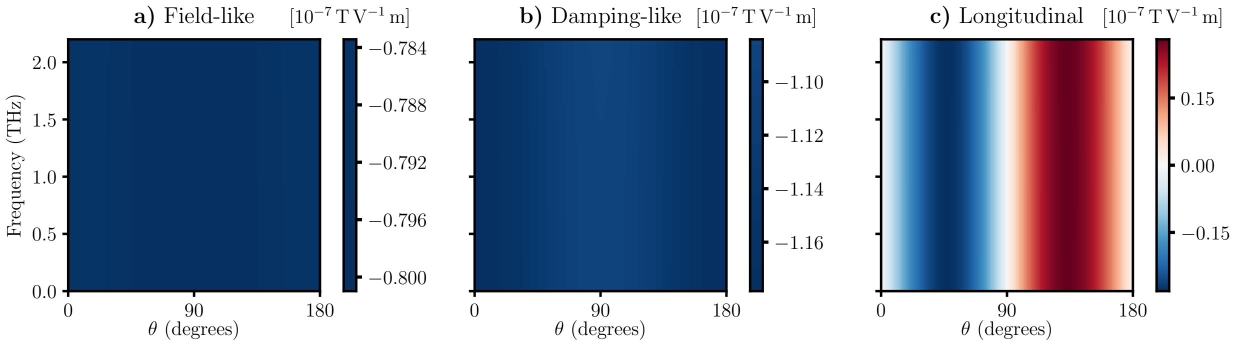


**Supplementary Figure 4** | Frequency and angular dependencies of the effective magnetic fields for the Co monolayer deposited on Pt(001). (a) Field-like, (b) Damping-like and (c) Longitudinal components of the effective field $\mathbf{B}_i^{\text{eff}}(\omega)$, given by Eq. (6) of the main text, in the local frame of reference that are in phase with the oscillatory electric field, when the magnetic moment of the ferromagnetic layer in the Co/Pt(100) bilayer is rotated within the $zx$ plane by an external magnetic field. As explained in the main text, the effective field is independent of the frequency in the investigated range. In this case, different than in Fe/W(110), the higher order contributions to the transverse components of the effective fields are small due to the higher symmetry of Co/Pt(001).

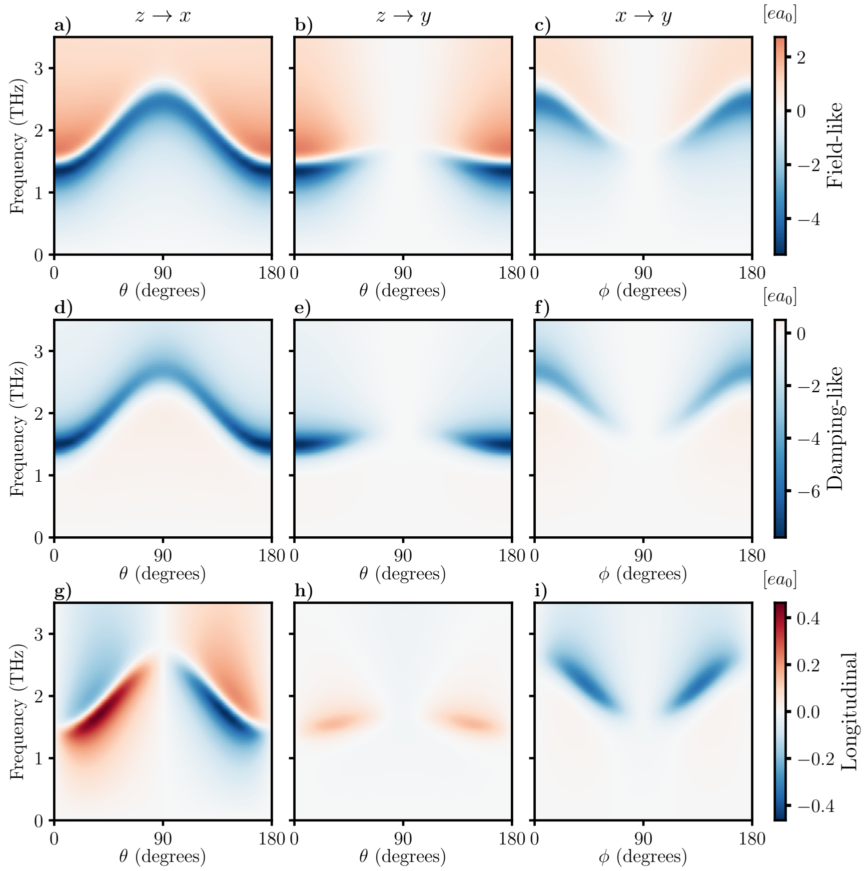


**Supplementary Figure 5** | Frequency and angular dependencies of the dynamical field-like (a-c), damping-like (d-f), and longitudinal (g-i) spin-orbit torques $\boldsymbol{\tau}^{\mathrm{SOT}}$, out-of-phase with the oscillatory electric field, when the magnetic moment of the ferromagnetic layer in the Fe/W(110) bilayer is rotated by an external magnetic field within the $zx$ plane (a,d,g), the $zy$ plane (b,e,h) and the $xy$ plane (c,f,i). The torques are obtained in units of $ea_0 = 8.48 \times 10^{-30}\,\mathrm{C\,m}$, where $e$ is the electronic charge and $a_0$ is the Bohr radius. The torque vector was decomposed into the local frame of reference given by: a field-like component along $\hat{\mathbf{m}}_{\mathrm{Fe}} \times \delta\hat{\mathbf{s}}$ (a,b,c); a damping-like component along $\hat{\mathbf{m}}_{\mathrm{Fe}} \times (\hat{\mathbf{m}}_{\mathrm{Fe}} \times \delta\hat{\mathbf{s}})$ (d,e,f); and a longitudinal contribution along $\hat{\mathbf{m}}_{\mathrm{Fe}}$ (g,h,i). The transverse components of the torque vanish for $\mathbf{M}_{\mathrm{Fe}} \| \delta\hat{\mathbf{s}} \| \hat{\mathbf{y}}$.

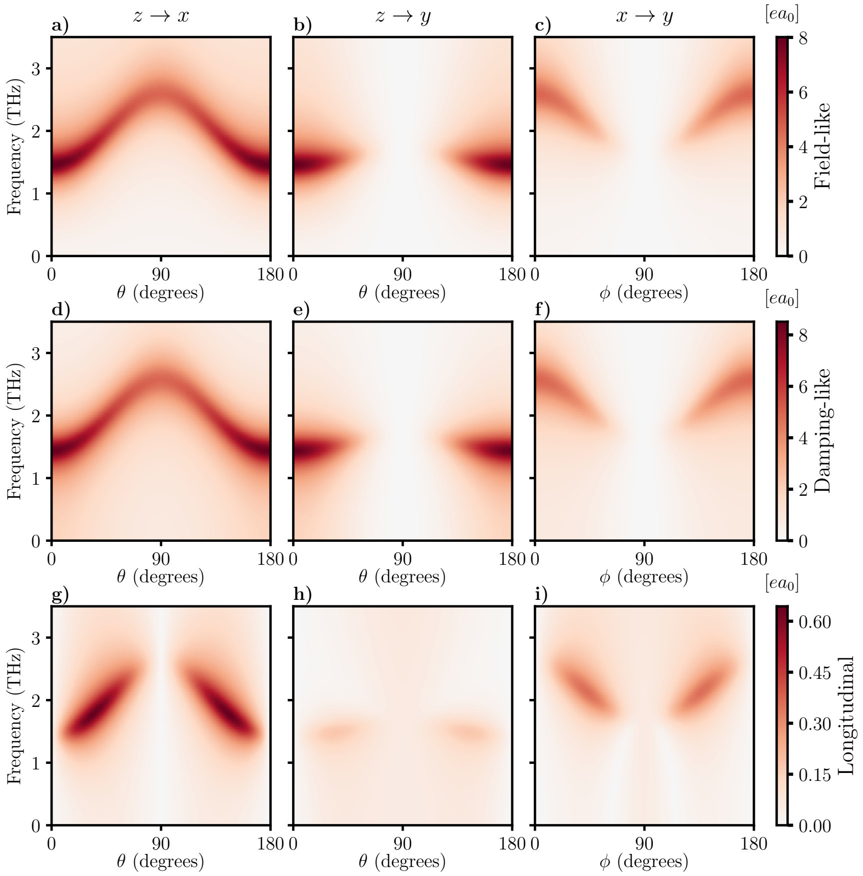


**Supplementary Figure 6** | Frequency and angular dependencies of the amplitude of the dynamical field-like (a-c), damping-like (d-f), and longitudinal (g-i) spin-orbit torques $|\tau^{\text{SOT}}_{i,\alpha}(\omega)| = \sqrt{\tau^{\text{in-phase}}_{i,\alpha}(\omega)^2 + \tau^{\text{out-phase}}_{i,\alpha}(\omega)^2}$, when the magnetic moment of the ferromagnetic layer in the Fe/W(110) bilayer is rotated by an external magnetic field within the $zx$ plane (a,d,g), the $zy$ plane (b,e,h) and the $xy$ plane (c,f,i). The torques are obtained in units of $ea_0 = 8.48 \times 10^{-30}\,\text{C m}$, where $e$ is the electronic charge and $a_0$ is the Bohr radius. The field-like and damping-like components follow similar behavior as a function of the frequency close to the resonance, leading to the featureless ratio of their amplitudes shown in Fig. 4c of the main text.

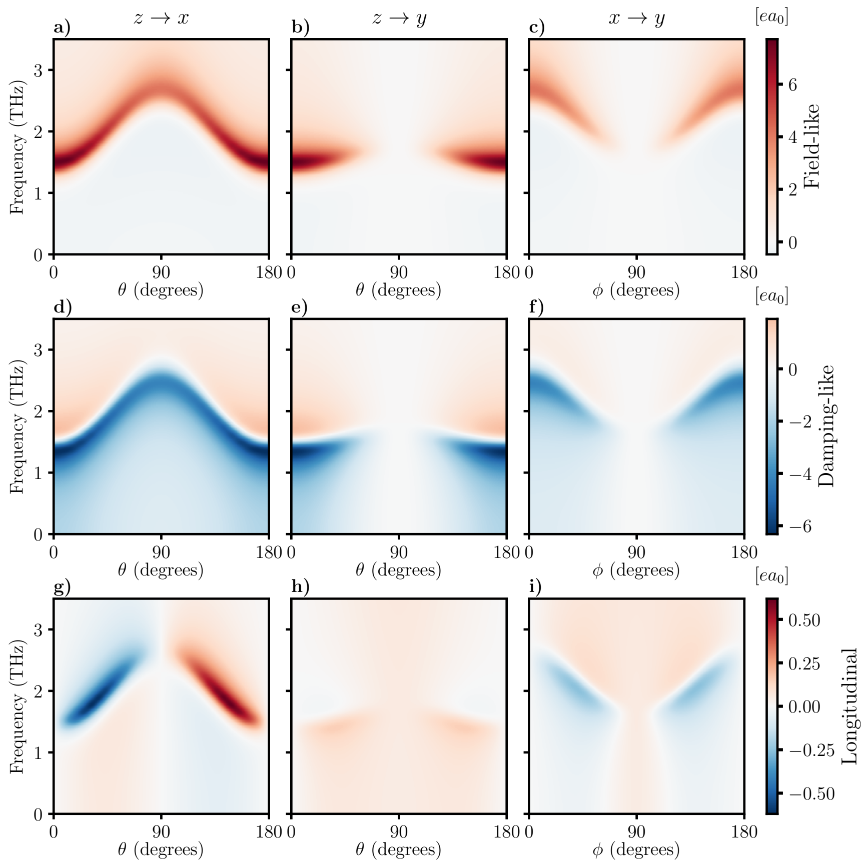


**Supplementary Figure 7** | Frequency and angular dependencies of the dynamical field-like (a-c), damping-like (d-f), and longitudinal (g-i) spin-orbit torques $\boldsymbol{\tau}^{\mathrm{SOT}}$, in-phase with the oscillatory electric field, when the magnetic moment of the ferromagnetic layer in the Fe/W(110) bilayer is rotated by an external magnetic field within the $zx$ plane (a,d,g), the $zy$ plane (b,e,h) and the $xy$ plane (c,f,i). The torques are obtained in units of $ea_0 = 8.48 \times 10^{-30}\,\mathrm{C\,m}$, where $e$ is the electronic charge and $a_0$ is the Bohr radius. The torque vector was decomposed into the local frame of reference given by: a field-like component along $\hat{\mathbf{m}}_{\mathrm{Fe}} \times \delta\hat{\mathbf{s}}$ (a,b,c); a damping-like component along $\hat{\mathbf{m}}_{\mathrm{Fe}} \times (\hat{\mathbf{m}}_{\mathrm{Fe}} \times \delta\hat{\mathbf{s}})$ (d,e,f); and a longitudinal contribution along $\hat{\mathbf{m}}_{\mathrm{Fe}}$ (g,h,i). The transverse components of the torque vanish for $\mathbf{M}_{\mathrm{Fe}} \| \delta\hat{\mathbf{s}} \| \hat{\mathbf{y}}$.

| System | Component | Plane | Order 0 | Order 2 | Order 4 |
|---|---|---|---|---|---|
| Fe/W(110) | $B_\theta$ | $zx$ | -0.0544 | -0.1034 | 0.0075 |
| | | $zy$ | 0.8637 | -0.0371 | -0.0074 |
| | $B_\phi$ | $zx$ | 0.8631 | 0.0242 | -0.0112 |
| | | $zy$ | -0.0544 | 0.0431 | 0.0005 |
| | $B_r$ | $zx$ | -0.3221 | 0.1003 | -0.0113 |
| | | $zy$ | -2.9261 | 0.0124 | 0.0369 |
| Co/Pt(001) | $B_\theta$ | $zx$ | 0.7839 | 0.0274 | -0.0100 |
| | | $zy$ | -1.1787 | 0.1169 | -0.0164 |
| | $B_\phi$ | $zx$ | -1.1786 | 0.0891 | 0.0016 |
| | | $zy$ | 0.7848 | -0.0705 | 0.0330 |
| | $B_r$ | $zx$ | -0.5348 | -0.0134 | -0.0695 |
| | | $zy$ | 6.3369 | -0.4112 | 0.2578 |

**Supplementary Table 1 |** Parameters for the effective fields generated in Fe/W(110) and Co/Pt(001) obtained by fitting Equations (22) – (24) to the calculated results. All values are given in units of $10^{-7}\,\mathrm{T\,V^{-1}\,m}$.

## SUPPLEMENTARY NOTES

### Supplementary Note 1 | Theoretical approach

In this Note, we use hats to denote operators instead of unit vectors.

**Ground state** The system is described by the Hamiltonian

$$\hat{H} = \hat{H}^0 + \hat{H}^{\mathrm{Z}} + \hat{H}^{\mathrm{SOI}} + \hat{H}^{\mathrm{int}} \quad . \tag{1}$$

where

$$\hat{H}_0 = \frac{1}{N} \sum_{\sigma} \sum_{ij\mu\nu} t_{ij}^{\mu\nu} \hat{c}^{\dagger}_{i\mu\sigma} \hat{c}_{j\nu\sigma} \quad , \tag{2}$$

is the tight-binding Hamiltonian describing the electronic hoppings, with $\hat{c}^{\dagger}_{i\mu\sigma}$ and $\hat{c}_{j\nu\sigma}$ being the creation and annihilation operators of electrons with spin $\sigma$ in the orbitals $\mu$ of site $i$ and $\nu$ of site $j$, respectively. The hopping matrices $t_{ij}^{\mu\nu}$ up to second nearest neighbors are obtained from density functional calculations based on the real-space linear-muffin tin orbitals method, within the atomic sphere approximation (RS-LMTO-ASA) [1–3].

The interaction with a uniform static external magnetic field $\mathbf{B}^{\mathrm{ext}}$ is described by

$$\hat{H}^{\mathrm{Z}} = \sum_{\substack{i\mu\nu \\ \sigma\sigma'}} \sum_{\alpha} B_{\alpha}^{\mathrm{ext}} (L_{\mu\nu}^{\alpha} \delta_{\sigma\sigma'} + 2S_{\sigma\sigma'}^{\alpha} \delta_{\mu\nu}) \hat{c}^{\dagger}_{i\mu\sigma} \hat{c}_{i\mu\sigma'} \quad , \tag{3}$$

where $\hbar = \mu_{\mathrm{B}} = 1$ (atomic units) and we used $g_{\mathrm{L}} = 1$ and $g_{\mathrm{S}} = 2$ as the Landé factors for the orbital and spin angular momentum.

The coupling between the spin and orbital degrees of freedom are included through an atomic spin-orbit interaction described by

$$\hat{H}^{\mathrm{SOI}} = \sum_{\substack{i\mu\nu \\ \sigma\sigma'}} \sum_{\alpha} \lambda_i L^{\alpha}_{\mu\nu} S^{\alpha}_{\sigma\sigma'} \hat{c}^{\dagger}_{i\mu\sigma} \hat{c}_{i\nu\sigma'} \quad , \tag{4}$$

where $L^{\alpha}$ and $S^{\alpha}$ are the $\alpha$ components of the orbital and spin angular momentum operators, respectively. The magnitudes of the SOI $\lambda_i$ for the different sites $i$ are also obtained from first-principles calculations.

Finally, the electron-electron interaction is characterized by a local Hubbard-like [4] interaction within the Lowde-Windsor approximation [5,6], including both direct and exchange contributions. For the ground state, we treat this interaction within the mean-field approximation, resulting in the exchange-correlation term

$$\hat{H}_{\text{int}} = -\sum_{\substack{i,\mu\in d \\ \sigma\sigma'}} \sum_{\alpha} U_i M^{\alpha}_i S^{\alpha}_{\sigma\sigma'} \hat{c}^{\dagger}_{i\mu\sigma} \hat{c}_{i\mu\sigma'} \ . \tag{5}$$

Here, $U_i$ is the local effective Coulomb interaction at site $i$, $M^{\alpha}_i$ and $S^{\alpha}$ are the $\alpha$-components of the magnetic moment vector and of the spin operator, respectively. We use $U_i = 1.0\,\mathrm{eV}$ for Fe, Co and W, and $U_i = 0.6\,\mathrm{eV}$ for Pt [7–9]. The magnetic moment in each atom $i$ is obtained as

$$\mathbf{M}_i = -\langle \hat{\boldsymbol{\sigma}} \rangle_i = \frac{1}{\pi} \mathrm{Im} \int_{-\infty}^{E_F} \mathrm{d}E \, \mathrm{Tr} \, G_{ii}(E + \mathrm{i}\Gamma) \, \hat{\boldsymbol{\sigma}} \tag{6}$$

in a self-consistent fashion, assuming a fixed value of the Fermi energy and adjusting the occupation of the $d$-orbitals to reproduce the DFT calculations. The trace in Eq. (6) is done over orbitals and spins. A constant broadening of $\Gamma = 68\,\mathrm{meV}$ is used in the single-particle Green function, $\hat{G}(E) = \left(E - \hat{H}\right)^{-1}$.

**Excitations** The magnetic moments are excited by a uniform and oscillatory electric field given by $\mathbf{E}(t) = E_0 \cos(\omega t)\, \mathbf{u}_E$, where $E_0$ and $\mathbf{u}_E$ are the amplitude and the direction of $\mathbf{E}$, respectively. Up to linear order in the applied electric field, the perturbation Hamiltonian can be written in terms of the vector potential $\mathbf{A}(t) = \int^t \mathbf{E}(t')\, \mathrm{d}t'$ as

$$\begin{aligned}\hat{H}^{\text{pert}}(t) =& -\int \mathrm{d}\mathbf{r}\, \hat{\mathbf{J}}^{\mathrm{C}}(\mathbf{r}, t) \cdot \mathbf{A}(t) \\ =& \frac{eE_0}{m\omega} \sum_{\sigma} \sum_{\substack{ij \\ \mu\nu}} \mathbf{p}_{ij}^{\mu\nu} \cdot \mathbf{u}_E \sin(\omega t) \hat{c}_{i\mu\sigma}^{\dagger}(t) \hat{c}_{j\nu\sigma}(t) \quad .\end{aligned} \tag{7}$$

where $\hat{\mathbf{J}}^{\mathrm{C}}(\mathbf{r}, t)$ is the current density operator, $e$ and $m$ are the electronic charge and mass, respectively, and $\mathbf{p}_{ij}^{\mu\nu} \cdot \mathbf{u}_E$ is the matrix element of the linear momentum vector operator in the direction of the electric field, $\mathbf{u}_E$. The time dependence of the fermionic operators is given by the unperturbed hamiltonian.

The external electrical perturbation causes a disturbance in the magnetic moments $\mathbf{M}_i \to \mathbf{M}_i + \delta\mathbf{M}_i(t)$, where $\delta\mathbf{M}_i(t)$ is linear in the electric perturbation (see Eq. (5) in the main text) and originates from the spin-orbit interaction. Therefore, the electron-electron interaction given in Eq. (5) will also give rise to a change in the total Hamiltonian

$$\begin{aligned}\delta\hat{H}^{\text{int}}(t) =& -\sum_{\substack{i,\mu\in d \\ \sigma\sigma'}} \sum_{\alpha} U_i \delta M_i^{\alpha}(t) S_{\sigma\sigma'}^{\alpha} \hat{c}_{i\mu\sigma}^{\dagger} \hat{c}_{i\mu\sigma'} \\ =& -\sum_{\substack{ij,\mu\in d \\ \sigma\sigma'}} \sum_{\alpha,\beta} U_i \int \mathrm{d}t'\, \Xi_{ij}^{\alpha\beta}(t-t') A_j^{\beta}(t') S_{\sigma\sigma'}^{\alpha} \hat{c}_{i\mu\sigma}^{\dagger} \hat{c}_{i\mu\sigma'} \;.\end{aligned} \tag{8}$$

where $\Xi_{ij}(t-t')$ represents the magnetic-charge current response, as defined in the main text. The total perturbed Hamiltonian is then given by $\hat{H}^{\text{total}} = \hat{H} + \delta\hat{H}^{\text{int}}(t) + \hat{H}^{\text{pert}}(t)$.

*Linear response* — We access the torques caused by the electric field using linear response

theory [10]. The variation in the $\alpha$ component of the torque acting on the spin magnetic moment of site $i$, $\tau_{i,\alpha}$, due to the application of the external perturbation is given by

$$\delta\langle\hat{\tau}_{i,\alpha}\rangle(t) = -\mathrm{i}\int dt'\langle[\hat{\tau}_{i,\alpha}(t), \hat{H}^{\mathrm{pert}}(t')]\rangle + \langle\delta\hat{\tau}_{i,\alpha}\rangle\ . \tag{9}$$

While the first term involves the response function of the torque due to the electric field, the second term originates in the change of the torque operator $\hat{\tau}_{i,\alpha}$ caused by the application of the electric field. It is analogous to the diamagnetic contribution to the electric current, obtained as the charge current evaluated in the ground state.

The torque operator $\hat{\boldsymbol{\tau}}_i$ as well as the spin current flowing from site $i$ to site $j$, $\hat{\mathbf{I}}^{\mathrm{S}}_{ij}$, are defined from the continuity equation. The evolution of the spin magnetic moment in the presence of the electric field can be described in the Heisenberg picture through the equation of motion of the spin operator,

$$\frac{\mathrm{d}\hat{\mathbf{S}}_i}{\mathrm{d}t} = -\sum_j \hat{\mathbf{I}}^{\mathrm{S}}_{ij} + \hat{\boldsymbol{\tau}}_i = -\mathrm{i}\,[\hat{\mathbf{S}}_i, \hat{H} + \delta\hat{H}^{\mathrm{int}}(t) + \hat{H}^{\mathrm{pert}}(t)] \quad . \tag{10}$$

The spin current flowing out of site $i$ is obtained from the tight-binding Hamiltonian given in Eq. 2, $\sum_j \hat{\mathbf{I}}^{\mathrm{S}}_{ij} = [\hat{\mathbf{S}}_i, \hat{H}^0]$. The torque operator $\hat{\boldsymbol{\tau}}_i$ can be separated into different contributions:

$$\begin{aligned}\hat{\boldsymbol{\tau}}_i =& [\hat{\mathbf{S}}_i, \hat{H}^{\mathrm{Z}} + \hat{H}^{\mathrm{SOI}} + \hat{H}^{\mathrm{int}} + \delta\hat{H}^{\mathrm{int}}(t)] \\ =& \hat{\boldsymbol{\tau}}^{\mathrm{Z}}_i + \hat{\boldsymbol{\tau}}^{\mathrm{SOI}}_i + \hat{\boldsymbol{\tau}}^{\mathrm{int}}_i + \delta\hat{\boldsymbol{\tau}}^{\mathrm{int}}_i(t)\end{aligned} \quad . \tag{11}$$

They represent, respectively: the Zeeman torque due to the external magnetic field,

$$\hat{\boldsymbol{\tau}}^{\mathrm{Z}}_i = 2\,\hat{\mathbf{S}}_i \times \mathbf{B}^{\mathrm{ext}}\ , \tag{12}$$

the local spin-orbit torque,

$$\hat{\boldsymbol{\tau}}^{\mathrm{SOI}}_i = \lambda_i\,\hat{\mathbf{S}}_i \times \hat{\mathbf{L}}_i \tag{13}$$

and the exchange correlation torque, given by the two terms

$$\hat{\boldsymbol{\tau}}_i^{\text{int}} = U_i\,\hat{\mathbf{S}}_i \times \mathbf{M}_i \quad \text{and} \quad \delta\hat{\boldsymbol{\tau}}_i^{\text{int}}(t) = U_i\,\hat{\mathbf{S}}_i \times \delta\mathbf{M}_i(t)\ . \tag{14}$$

The total exchange torque caused by the electric field is obtained by substituting the operators given by Eq. (14) into Eq. (9),

$$\delta\langle\hat{\boldsymbol{\tau}}_i^{\text{int}}\rangle = -\,U_i\left[\delta\langle\hat{\mathbf{S}}_i\rangle(t) \times \mathbf{M}_i + \langle\hat{\mathbf{S}}_i\rangle \times \delta\mathbf{M}_i(t)\right] \quad . \tag{15}$$

The first term involves the response of the spins caused by the external perturbation, with $\delta\mathbf{M}_i(t) = -2\delta\langle\hat{\mathbf{S}}_i\rangle(t)$. The second term, given by the expectation value of $\delta\hat{\boldsymbol{\tau}}_i^{\text{int}}(t)$, is already proportional to the change in the magnetic moment caused by the electric field, $\delta\mathbf{M}_i(t) = \sum_j \int \mathrm{d}t'\,\Xi_{ij}(t - t')\,\mathbf{A}_j(t')$. This, in our linear response approach, must be calculated in the ground state, such that $-2\langle\hat{\mathbf{S}}_i\rangle = \mathbf{M}_i$. Therefore, these terms cancel identically, and $\delta\langle\hat{\boldsymbol{\tau}}_i^{\text{int}}\rangle = 0$. Such result is expected within our framework where the exchange field is proportional to the spin magnetic moment.

The remaining term, $[\hat{\mathbf{S}}_i, \hat{H}^{\text{pert}}(t)]$, is proportional to $\mathbf{A}(t) = \frac{E_0}{\omega}\sin(\omega t)\mathbf{u}_E$. Note that this term is linear in the external field, and its expectation value, taken in the ground state, gives rise to an out-of-phase contribution that diverges as $1/\omega$. This term is cancelled in the static limit by the out-of-phase contribution from the first term in Eq. (9) (as described in the case of charge currents in Supplementary Ref. 6).

## Supplementary Note 2 | Renormalization factor in the effective magnetic fields

In this Note, we show, in some mathematical detail, why the renormalization factor due to the electron-electron interactions cancels out in the definition of the effective magnetic fields, Eq. (6) in the main text.

The general double-time retarded response function can be written in the time domain as

$$\mathcal{X}^{XY}(t) = \langle\langle \hat{X}(t), \hat{Y} \rangle\rangle = -\mathrm{i}\Theta(t)\langle \hat{X}(t), \hat{Y} \rangle \ , \tag{16}$$

where $\Theta(t)$ is the Heaviside step function. We can write the single-particle operators in second quantization to obtain the most general form for this response as

$$\mathcal{X}^{XY}_{pq,rs}(t) = -\mathrm{i}\Theta(t) X_{pq} \langle [\hat{c}^\dagger_p(t)\hat{c}_q(t), \hat{c}^\dagger_r \hat{c}_s] \rangle Y_{rs} \ , \tag{17}$$

where $p, q, r, s$ denotes a general basis in which the operator components are given by $X_{pq} = \langle p|\hat{X}|q\rangle$ and $Y_{rs} = \langle r|\hat{Y}|s\rangle$. In our case, we use the tight binding basis composed by sites $i$, orbital $\mu$ and spins $\sigma$ so that, e.g., $p \to \{i, \mu, \sigma\}$. We can now define a general response tensor, from which all possible response functions can be calculated, as

$$\mathcal{X}_{pq,rs}(t) = -\mathrm{i}\Theta(t)\langle [\hat{c}^\dagger_p(t)\hat{c}_q(t), \hat{c}^\dagger_r \hat{c}_s] \rangle \ , \tag{18}$$

such that

$$\mathcal{X}^{XY}_{pq,rs}(t) = X_{pq} \mathcal{X}_{pq,rs}(t) Y_{rs} \ . \tag{19}$$

In particular, for the cases described in the main text, $\hat{X} = \hat{S}^\alpha_i$, the $\alpha$-component of the spin operator at site $i$. $\hat{Y}$ is either $\hat{J}^{\mathrm{C},\beta}_{kl}$ (the $\beta$-component of the charge current density operator flowing

between sites $k$ and $l$) when an electric field is applied, or $\hat{S}_j^{\beta}$ when a magnetic field is applied. In the following, we introduce matrix notation $\underline{\mathcal{X}}$ with the rows given by the combined $\{p, q\}$ index and the columns by the combined $\{r, s\}$ index.

The desired quantities are calculated by solving their respective equation of motion in the frequency domain (for further details, see, e.g., Supplementary Ref. 11 and the Supplemental Material of the Supplementary Ref. 6). In matrix representation, this results in

$$\begin{aligned} \underline{\Xi}(\omega) &= \underline{\Xi}_0(\omega) - \underline{\chi}_0(\omega)\, \underline{U}\, \underline{\Xi}(\omega) \\ \underline{\chi}(\omega) &= \underline{\chi}_0(\omega) - \underline{\chi}_0(\omega)\, \underline{U}\, \underline{\chi}(\omega) \ . \end{aligned} \tag{20}$$

where $\underline{\Xi}$ is the magnetic-charge current response (spin density couples to charge current density) and $\underline{\chi}$ is the magnetic susceptibility (spin density couples to spin density), both renormalized by the electron-electron interaction $\underline{U}$, while $\underline{\Xi}_0$ and $\underline{\chi}_0$ are the respective bare responses. In both cases, the electron-electron interaction is renormalizing the response of the spin-density, which is why $\underline{\chi}_0(\omega)$ also appears in the first of these equations.

It is then follows that

$$\begin{aligned} [\underline{\chi}(\omega)]^{-1}\underline{\Xi}(\omega) &= [\underline{\chi}_0(\omega)]^{-1}(1 + \underline{\chi}_0(\omega)\underline{U})\ (1 + \underline{\chi}_0(\omega)\underline{U})^{-1}\underline{\Xi}_0(\omega) \\ &= [\underline{\chi}_0(\omega)]^{-1}\underline{\Xi}_0(\omega) \ , \end{aligned} \tag{21}$$

demonstrating that the renormalization factors cancels out.

## Supplementary Note 3 | Fits of the effective fields

To quantify the effective fields generated in Fe/W(110) and in Co/Pt(001) bilayers, we use the functional forms for their spherical components $\mathbf{B} = B_\theta(\theta,\phi)\mathbf{e}_\theta + B_\phi(\theta,\phi)\mathbf{e}_\phi + B_r(\theta,\phi)\mathbf{e}_r$ obtained by symmetry analysis in the Supplemental Material of Supplementary Ref. 12. Here $\mathbf{e}_r$, $\mathbf{e}_\theta$ and $\mathbf{e}_\theta$ are the standard unit vectors in the radial, polar and azimuthal directions, respectively. The components of the effective fields are given by:

$$\begin{aligned} B_\theta(\theta,\phi) = &\cos\phi\left(A_0^\phi + A_2^\phi \sin^2\theta + A_4^\phi \sin^4\theta + \cdots\right) \\ &+ \cos\theta\sin\phi\left(-A_0^\theta + B_2^\phi \sin^2\theta + B_4^\phi \sin^4\theta + \cdots\right) \ , \end{aligned} \tag{22}$$

$$\begin{aligned} B_\phi(\theta,\phi) = &- \cos\phi\left(A_0^\theta + A_2^\theta \sin^2\theta + A_4^\theta \sin^4\theta + \cdots\right) \\ &- \cos\theta\sin\phi\left(A_0^\phi + B_2^\theta \sin^2\theta + B_4^\theta \sin^4\theta + \cdots\right) \ , \end{aligned} \tag{23}$$

$$\begin{aligned} B_r(\theta,\phi) = &\sin\theta\cos\theta\cos\phi\left(A_0^r + A_2^r \sin^2\theta + A_4^r \sin^4\theta + \cdots\right) \\ &+ \sin\theta\sin\phi\left(B_0^r + B_2^r \sin^2\theta + B_4^r \sin^4\theta + \cdots\right) \ . \end{aligned} \tag{24}$$

We use the formulas above to fit the effective fields, and the obtained parameters are listed in Table 1. The effective field in the local frame of reference can be written in terms of the above

components as

$$\begin{aligned}\mathbf{B}^{\mathrm{FL}}(\theta,\phi) =& \cos\phi(A_0^\phi + A_2^\phi \sin^2\theta + A_4^\phi \sin^4\theta + \cdots)\mathbf{e}_\theta \\ & - \cos\theta\sin\phi(A_0^\phi + B_2^\theta \sin^2\theta + B_4^\theta \sin^4\theta \cdots)\mathbf{e}_\phi \ ,\end{aligned} \tag{25}$$

$$\begin{aligned}\mathbf{B}^{\mathrm{DL}}(\theta,\phi) =& -\cos\phi(A_0^\theta + A_2^\theta \sin^2\theta + A_4^\theta \sin^4\theta + \cdots)\mathbf{e}_\phi \\ & + \cos\theta\sin\phi(-A_0^\theta + B_2^\phi \sin^2\theta + B_4^\phi \sin^4\theta \cdots)\mathbf{e}_\theta\end{aligned} \ . \tag{26}$$

For Fe/W(110), $A_2^\phi > A_0^\phi$, leading to the large variation in the field-like component displayed in Fig. 5a of the main text.

**Supplementary References**


1. Andersen, O. K. & Jepsen, O. Explicit, First-Principles Tight-Binding Theory. *Phys. Rev. Lett.* **53**, 2571–2574 (1984).

2. Peduto, P. R., Frota-Pessôa, S. & Methfessel, M. S. First-principles linear muffin-tin orbital atomic-sphere approximation calculations in real space. *Phys. Rev. B* **44**, 13283–13290 (1991).

3. Frota-Pessôa, S. First-principles real-space linear-muffin-tin-orbital calculations of 3*d* impurities in Cu. *Phys. Rev. B* **46**, 14570–14577 (1992).

4. Hubbard, J. Electron Correlations in Narrow Energy Bands. *Proceedings of the Royal Society A: Mathematical, Physical and Engineering Sciences* **276**, 238–257 (1963).

5. Lowde, R. D. & Windsor, C. G. On the magnetic excitations in nickel. *Advances in Physics* **19**, 813–909 (2006).

6. Guimarães, F. S. M. *et al.* Dynamical amplification of magnetoresistances and Hall currents up to the THz regime. *Sci. Rep.* **7**, 3686 (2017).

7. Janak, J. F. Uniform susceptibilities of metallic elements. *Phys. Rev. B* **16**, 255–262 (1977).

8. Himpsel, F. J. Correlation between magnetic splitting and magnetic moment for 3d transition metals. *J. Magn. Magn. Mater.* **102**, 261–265 (1991).

9. Şaşıoğlu, E., Friedrich, C. & Blügel, S. Effective Coulomb interaction in transition metals from constrained random-phase approximation. *Phys. Rev. B* **83**, 121101 (2011).

10. Kubo, R. Statistical-Mechanical Theory of Irreversible Processes. I. General Theory and Simple Applications to Magnetic and Conduction Problems. *J. Phys. Soc. Jpn.* **12**, 570–586 (1957).

11. Costa, A. T., Muniz, R. B., Lounis, S., Klautau, A. B. & Mills, D. L. Spin-orbit coupling and spin waves in ultrathin ferromagnets: The spin-wave Rashba effect. *Phys. Rev. B* **82**, 014428 (2010).

12. Garello, K. *et al.* Symmetry and magnitude of spin-orbit torques in ferromagnetic heterostructures. *Nat. Nanotechnol.* **8**, 587–593 (2013).
